# Supplementary material for: Quantum Port: Gamification of quantum teleportation for public engagement
Source: arXiv:2503.22701 ancillary file (2026-03-31)
Supplement: Supplementary file 1 [file Game_rules.pdf]

## Game rules

1. There are two types of cards: **Circuit Cards** and **Action Cards**.
2. Before the game begins, select one (for **Beginner** setup) or two (for **Default** setup) **Quantum Data Coins (QDC)**.
3. Shuffle your deck and draw four cards on top of your deck. If you are unsatisfied with your hand, put your cards back, reshuffle, and redraw four cards on top of your deck. You can only reshuffle once.
4. Position the **QDC** and **Classical Coin** with the head facing down on your left.
5. This game is divided into two parts. The first part is to build a complete **Quantum Teleportation Circuit (QTC)** from your left to right, while the second part is to advance your **Classical Data Coin (CDC)**.
6. There are two types of **Circuit Cards**, i.e. the Black Thick (**Quantum**) circuits and White Thin (**Classical**) circuits.
7. The Black Thick circuits must begin with **Entangler** and end with **Pauli Correction**.
8. There is no restriction on the White Thin circuits as long as it is connected with the same number of cards as the Black Thick circuits.
9. Black Thick and White Thin circuit cards must be connected properly with the **QDC** and **Classical Coin** respectively.
10. Once the circuits are built, roll the dice and refer to the **Dice Rules** to decide which **CDC** to advance. Position your **CDC** with the head facing down on the first White Thin circuit card.
11. Once the **CDC** advances beyond the last White Thin circuit card, **QDC** will be teleported.
12. If the deck is expended, reshuffle the discarded deck and reuse the deck.
13. Win conditions
  - (a) One **QDC**: The fastest player to teleport the **QDC** wins
  - (b) Two **QDC**: The player with the most **QDC** wins

## Eligible **Turns** and **Moves**

Each player has two **Moves** per **Turn**. The following takes one **Move**.

1. Draw a card from the deck
2. Use a circuit card to build **QTC**
3. Discard a circuit card in the **QTC**
4. Use an **Action Card**
5. Roll the **Four-Sided Die** to decide the appropriate **CDC**
6. Advance the **CDC** one White Thin circuit card forward

A player can only have maximum four cards in hand. At the end of the turn, discard excess cards in hand. This does not count as one **Move**.

## Dice rules

| <b>CDC</b><br><b>QDC</b> | 00 | 01 | 10 | 11 |
|--------------------------|----|----|----|----|
| $\Psi^+$                 | 1  | 4  | 2  | 3  |
| $\Psi^-$                 | 2  | 3  | 1  | 4  |
| $\Phi^+$                 | 4  | 1  | 3  | 2  |
| $\Phi^-$                 | 3  | 2  | 4  | 1  |
