# Supplementary material for: Quantum Port: Gamification of quantum teleportation for public engagement
Source: arXiv:2503.22701 ancillary file (2026-03-31)

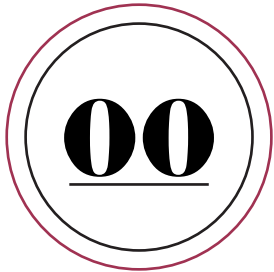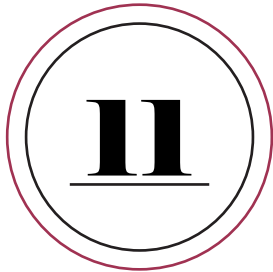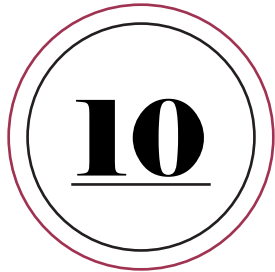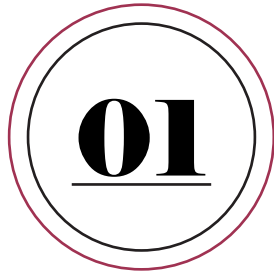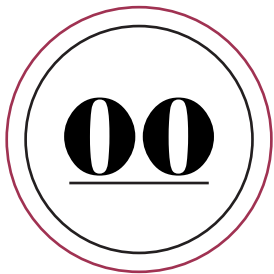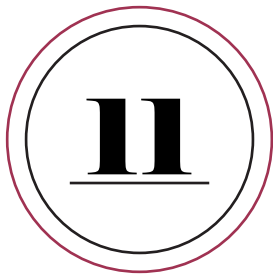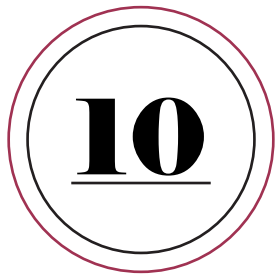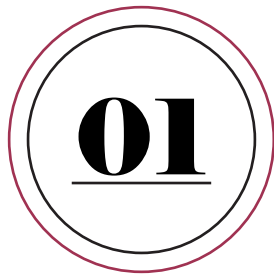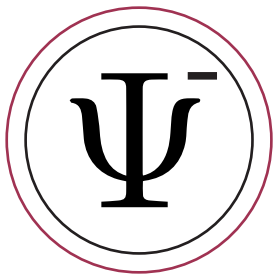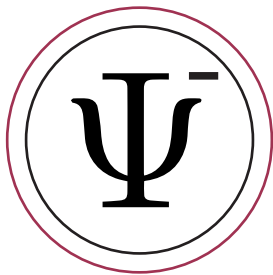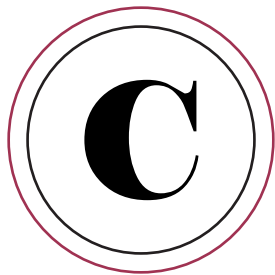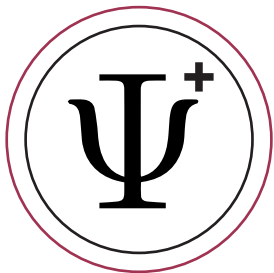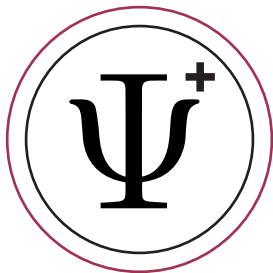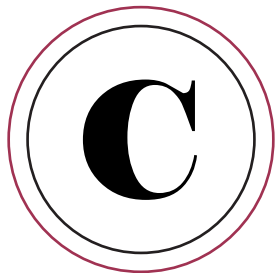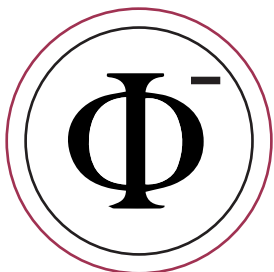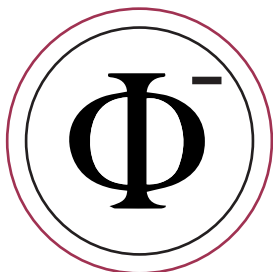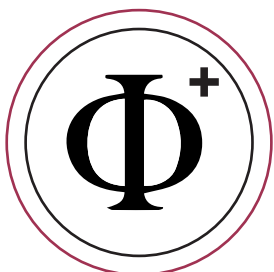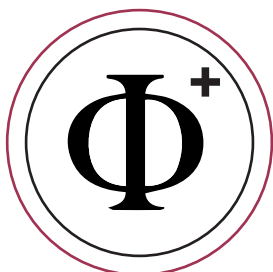

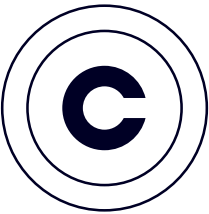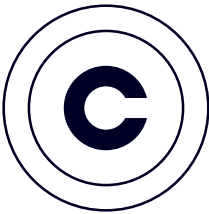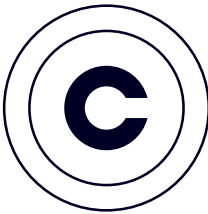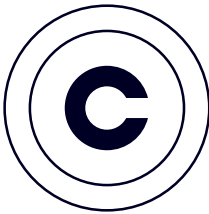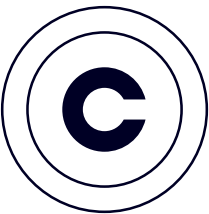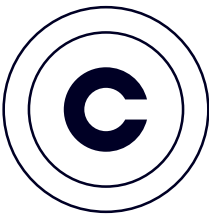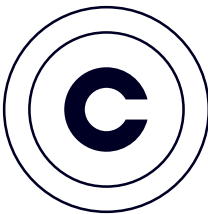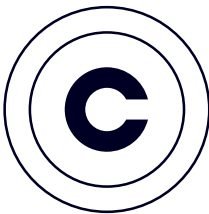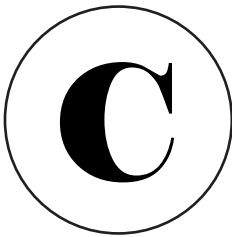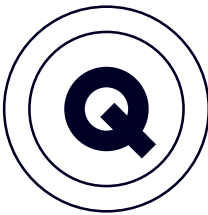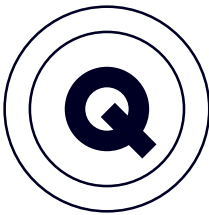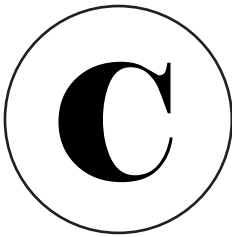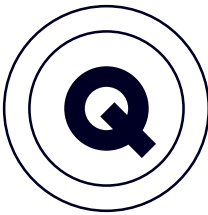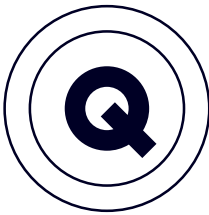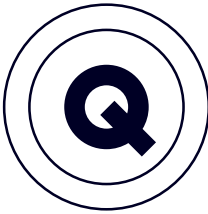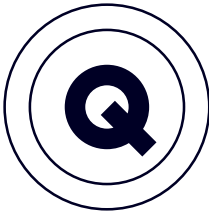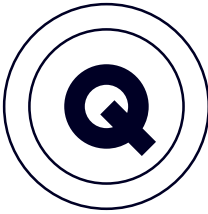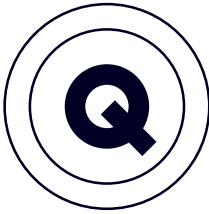

Supplement: Supplementary file 2 [file Quantum_Port_Coins.pdf]
